# Supplementary material for: Detection of radio emission from stars via proper-motion searches
Source: arXiv:2306.08059 source file (2023-06-13)
Supplement: Supplementary file 1 [file appendix_proper_motion.tex]

\section{Hospital Anxiety and Depression Scale (Italian Version)}

\section{Openness to Discuss Cancer in the Family Scale Questionario sulla Comunicazione in Famiglia (Italian Version)}

\begin{table}[hbt!]
\centering
\begin{threeparttable}
\caption{Predicting approval of one's own house member}\label{tab:predictapproval}
\begin{tabular}{lSSS}
  \toprule
   & {(1)} & {(2)} & {(3)} \\
   \midrule
   Religion Match & 0.077\tnote{***} & -0.029 & -0.027 \\
                  & {(0.014)} & {(0.061)} & {(0.062)} \\
   \bottomrule
\end{tabular}
\begin{tablenotes}[para]
  \item[]Note: Entries are coefficients from a probit regression model. Robust standard errors in parentheses.
  \item[***] $p < 0.01$,
  \item[**] $p < 0.05$,
  \item[*] $p < 0.1$, two-tailed test.
\end{tablenotes}
\end{threeparttable}
\end{table}
